# Supplementary material for: Unbiased Region-Language Alignment for Open-Vocabulary Dense Prediction
Source: arXiv:2412.06244 source file (2025-12-24)
Supplement: Supplementary file 1 [file base_novel.tex]

\begin{table*}[t]
  \tiny
  \centering
  \tablestyle{6pt}{1.}
  \caption{Split base and novel categories in ADE20K.
  }
  \label{tab: dataset-split}
%\vskip 0.15in
  \begin{center}
  \begin{small}
  % \begin{sc}
  \begin{tabular}{lc}
  \toprule
  Split & Name\\    
  \midrule
  \multirow{6}{*}{Base}  & \emph{wall, building, sky, floor, tree, ceiling, road, bed, windowpane, grass, cabinet, sidewalk,}\\
  &\emph{person, door, table, mountain, plant, curtain, chair, car, water, sofa, shelf, sea,}\\
  &\emph{mirror, rug, fence, rock, lamp, counter, sand, sink, refrigerator, stairs, pillow, river,} \\
  &\emph{bridge, toilet, flower, book, bench, palm tree, boat, bus, towel, light bulb, truck, } \\
  &\emph{television receiver, airplane, apparel, bottle, tent, oven, food, microwave, plant pots,} \\
  &\emph{animal, bicycle, blanket, vase, traffic light, plate, cup, clock} \\
  \midrule
  \multirow{10}{*}{Novel} & \emph{earth, painting, house exterior, field, armchair, seat, desk, wardrobe,}\\
  &\emph{bathtub, railing, cushion, pedestal, box, column, signboard, chest of drawers, skyscraper, }\\
  &\emph{fireplace, grandstand, path, runway, case, pool table, screen door, stairway, bookcase,}\\
  &\emph{window screen, coffee table, hill, countertop, stove, kitchen island, computer, swivel chair,}\\
  &\emph{arcade machine, hovel, tower, chandelier, awning, streetlight, booth, dirt track, pole, land,}\\
  &\emph{bannister, escalator, ottoman, buffet, poster, stage, van, ship, fountain, conveyer belt, }\\
  &\emph{washer, plaything, swimming pool, stool, barrel, basket, waterfall, bag, minibike, cradle, }\\
  &\emph{step, tank, trade name, lake, dishwasher, projection screen, sculpture, exhaust hood, sconce,  }\\
  &\emph{tray, ashcan, ceiling fan, pier, crt screen, monitor, bulletin board, shower, radiator,}\\
  &\emph{canopy, flag, bar,  ball }\\
 \bottomrule
  \end{tabular}
  % \end{sc}
  \end{small}
  \end{center}
  \vskip -0.1in
\end{table*}
