# Supplementary material for: Unbiased Region-Language Alignment for Open-Vocabulary Dense Prediction
Source: arXiv:2412.06244 source file (2025-12-24)
Supplement: Supplementary file 2 [file hyperparam.tex]

\begin{table*}[ht]
    % \vspace{30pt}
    \caption{Hyperparameter ablation study on ensembling of various branches.
    }
    % \vspace{-5pt}
    % \flushleft
    \centering
    \label{tab: hyperparameter}
    \captionsetup[subfloat]{labelformat=parens, labelsep=space, skip=1pt, position=top}
    \begin{minipage}{0.45\linewidth}
    \subfloat[Effect of ensembling original and additional mask prediction branches 
    on panoptic segmentation using the ADE20k.]{
    % \centering
    \small
    
    \setlength{\tabcolsep}{12.pt}
    \begin{tabularx}{1.0\textwidth}{l c c c}
    \toprule
     &PQ  & AP & mIoU\\
    \midrule
    $\alpha=0.0$ & 24.5 & 16.8 & 35.3 \\
    $\alpha=0.1$ & 25.8 & 17.0 & 35.6 \\
    $\alpha=0.2$ & 26.2 & 17.0 & 35.9 \\
    $\alpha=0.3$ & 26.7 & 16.9 & 36.2 \\
    $\alpha=0.4$ & 26.5 & 16.8 & 36.4 \\
    $\alpha=0.5$ & 26.8 & 16.7 & 36.4 \\
    \rowcolor{ourscolor}
    $\alpha=0.6$ & 27.0 & 16.6 & 36.5 \\
    $\alpha=0.7$ & 27.0 & 16.5 & 36.5 \\
    $\alpha=0.8$ & 26.7 & 16.5 & 36.4 \\
    $\alpha=0.9$ & 26.8 & 16.4 & 36.3 \\
    $\alpha=1.0$ & 26.7 & 16.4 & 36.2 \\
    % \rowcolor{ourscolor}
    \bottomrule
    \end{tabularx}}
  \end{minipage}
%   \vspace{7mm}
     \hspace{7mm}
     \begin{minipage}{0.4\linewidth}
      \subfloat[Effect of ensembling pixel prediction branch on ADE20K with 150 and 857 classes, 
      and Pascal Context with 459 classes.]{
    % \centering
    \small
    
    \setlength{\tabcolsep}{6.pt}
    \begin{tabularx}{1.0\textwidth}{l c c c}
      \toprule
       & A-150 & A-847 & PC-459\\
      \midrule
      $\beta=0.0$ & 34.5 & 15.1 & 19.9 \\
      $\beta=0.1$ & 34.9 & 15.2 & 20.0 \\
      $\beta=0.2$ & 35.5 & 15.4 & 20.2 \\
      $\beta=0.3$ &  35.8 & 15.4 & 20.5 \\
      $\beta=0.4$ &  36.2 & 15.4 & 20.7 \\
      \rowcolor{ourscolor}
      $\beta=0.5$ &  36.5 & 15.5 & 21.0 \\
      $\beta=0.6$ &  36.4 & 15.5 & 21.0 \\
      $\beta=0.7$ &  36.4 & 15.4 & 21.1 \\
      $\beta=0.8$ &  36.5 & 15.2 & 21.2 \\
      $\beta=0.9$ &  36.1 & 14.9 & 21.3 \\
      $\beta=1.0$ & 35.5 & 14.1 & 21.0\\
    \bottomrule
    \end{tabularx}}
    \end{minipage}
    %  \vspace{-15pt}
    \end{table*}
